# Supplementary material for: VITAL: More Understandable Feature Visualization through Distribution Alignment and Relevant Information Flow
Source: arXiv:2503.22399 source file (2026-02-17)
Supplement: Supplementary file 1 [file fig_method_sm_app.tex]

\begin{figure*}
    \centering
    \centerline{\includegraphics[width=\linewidth]
    {fig/method_sm_app.png}}
    \caption{\textbf{Overview of VITAL framework.} Our \ours framework consists of \bernt{the figure is huge - I doubt we will have the space for such a large figure}}
    \label{fig:fig_method_sm_app}

\end{figure*}
