# Supplementary material for: VITAL: More Understandable Feature Visualization through Distribution Alignment and Relevant Information Flow
Source: arXiv:2503.22399 source file (2026-02-17)
Supplement: Supplementary file 2 [file table_CLIP.tex]

\begin{table}[]
    \centering
    \begin{tabular}{cccc}
        \toprule
         Images & Setup & Top-1 ($\uparrow$) & Top-5 ($\uparrow$) \\ 
         \midrule
         ImageNet & clean & 69.11 & 92.23 \\
         \hdashline\noalign{\vskip 1.0ex}
         \multirow{2}{*}{MACO \cite{Fel2023}} & res: 224 & 12.87 & 29.73 \\
          & res: 1024 & 1.60 & 5.67\\
          \hdashline\noalign{\vskip 1.0ex}
         \multirow{2}{*}{Fourier} & res: 224 & 6.73 & 18.27\\
          & res: 1024 & 0.97 & 3.57\\
          \hdashline\noalign{\vskip 1.0ex}
          \multirow{2}{*}{CBR} & res: 224 & 0.20 & 1.17\\
          & res: 1024 & 0.20 & 1.07\\
          \hdashline\noalign{\vskip 1.0ex}
         \multirow{2}{*}{DeepInv \cite{yin2020dreaming}}& batch size: 64 & 29.90 & 55.20 \\
          & batch size: 1 & 4.73 & 12.63\\
         \hdashline\noalign{\vskip 1.0ex}
         DeepInv \cite{yin2020dreaming}& batch size: 64 & 17.20 & 40.43 \\
         down ($\downarrow2$) & batch size: 1 & 6.30 & 16.43 \\
         \midrule
         \textbf{VITAL} & - & 66.62 & 92.56\\
         \bottomrule
         
    \end{tabular}
    \caption{Caption}
    \label{tab:CLIP}
\end{table}
