# Supplementary material for: VITAL: More Understandable Feature Visualization through Distribution Alignment and Relevant Information Flow
Source: arXiv:2503.22399 source file (2026-02-17)
Supplement: Supplementary file 4 [file table_combined.tex]

\begin{table}[t]
    \centering
    \footnotesize
    \begin{tabular}{cccccc}
        \toprule
         \multirow{2}{*}{Method} & \multirow{2}{*}{Setup} &Acc. &  \multirow{2}{*}{FID ($\downarrow$)}& \multicolumn{2}{c}{Zero-Shot Prediction}   \\ 
         \cmidrule{5-6}%\cmidrule{6}
         & & Top1 ($\uparrow$) & & Top1 ($\uparrow$) & Top5 ($\uparrow$) \\
         \midrule
         ImageNet &  & - & -&  69.11 & 92.23 \\
         \hdashline\noalign{\vskip 1.0ex}
         \multirow{2}{*}{MACO} & r: 224 & 29.43 & 360.74 & 12.87 & 29.73 \\
         & r: 1024 & 2.10 & 494.57 & 1.60 & 5.67   \\
         \hdashline\noalign{\vskip 1.0ex}
         \multirow{2}{*}{Fourier} & r: 224 & 21.30 & 422.44 & 6.73 & 18.27  \\
         & r: 1024 & 3.43 & 430.58 & 0.97 & 3.57  \\
         \hdashline\noalign{\vskip 1.0ex}
         \multirow{2}{*}{CBR} & r: 224 & 0.50 & 545.50 & 0.20 & 1.17  \\
         & r: 1024 & 0.33 & 522.89 & 0.20 & 1.07  \\
         \hdashline\noalign{\vskip 1.0ex}
         \multirow{2}{*}{DeepInv}& bs: 64 & \textbf{100.00} & \textbf{35.76} & \textcolor{blue}{\textbf{29.90}} & \textcolor{blue}{\textbf{55.20}} \\
         & bs: 1 & \textbf{100.00} & 123.77 & 4.73 & 12.63  \\
         \hdashline\noalign{\vskip 1.0ex}
         DeepInv & bs: 64 & 50.47 & 176.35 & 17.20 & 40.43  \\
         ($\downarrow2$) & bs: 1 & \textbf{100.00} & 121.94 & 6.30 & 16.43  \\
         \midrule
         \textbf{VITAL} &  & \textcolor{blue}{\textbf{99.90}} & \textcolor{blue}{\textbf{58.79}} & \textbf{66.62} & \textbf{92.56}  \\
         \bottomrule
    \end{tabular}
    \caption{Comparison of methods on ResNet50 trained on Imagenet. We provide FID scores, CLIP Zero-shot prediction scores, and top-1 classification accuracy, indicating the \textbf{best} and \textcolor{blue}{\textbf{second best}}. In the settings, "r" indicates the resolution of the visualization and "bs" is the used batch size and indicate with ($\downarrow 2$) the multi-resolution optimization version of DeepInv.}
    \label{tab:combined}
\end{table}
